# Supplementary material for: Did the Musk Takeover Boost Contentious Actors on Twitter?
Source: arXiv:2212.10646 source file (2022-12-20)
Supplement: Supplementary file 1 [file resources.tex]

\section{Key resources}

\begin{table}
\centering
\begin{tabular}[t]{lcc}
\toprule
  & Retweets & Likes\\
\midrule
Paid verification & \num{-0.063} & \num{-0.077}***\\
 & (\num{0.046}) & (\num{0.018})\\
Musk acquisition & \num{0.132}*** & \num{0.003}\\
 & (\num{0.035}) & (\num{0.013})\\
Tweets (logged sum) & \num{1.952}*** & \num{1.315}***\\
 & (\num{0.032}) & (\num{0.014})\\
\midrule
Observations & \num{183801} & \num{183801}\\
User fixed effect & X & X\\
Year-month fixed effect & X & X\\
\bottomrule
\multicolumn{3}{l}{\rule{0pt}{1em}Standard errors clustered by user}\\
\multicolumn{3}{l}{\rule{0pt}{1em}Outcomes are logged retweets and likes}\\
\multicolumn{3}{l}{\rule{0pt}{1em}* p $<$ 0.05, ** p $<$ 0.01, *** p $<$ 0.001}\\
\end{tabular}
\end{table}
